# Supplementary material for: On Positivity and Minimality for Second-Order Holonomic Sequences
Source: arXiv:2007.12282 source file (2020-07-23)
Supplement: Supplementary file 1 [file Appendix_oracle_reductions.tex]

\section{Oracle reductions}

Let \((u_n)_{n=-1}^\infty\) be a non-trivial solution of the recurrence relation \(u_n =b_nu_{n-1} + a_nu_{n-2}\).  If \(u_{n-1}\neq 0\) then we can rearrange the relation to obtain
	\begin{equation*}
		-\frac{u_{n-1}}{u_{n-2}} = \frac{a_n}{b_n - \frac{u_n}{u_{n-1}}}
	\end{equation*}
for \(n\in\N\).
In the event that \(u_{n-2}=0\) we take the usual interpretation in \(\hat{\C}\).
Since \((u_n)\) is non-trivial  and \(a_n\neq 0\) for each \(n\in\N\), the sequence \((u_n)\) does not vanish at two consecutive indices.
Thus if \(u_{n-1}=0\) then \(u_{n-2},u_n\neq 0\) and so both the left-hand the right-hand sides of the last equation are well-defined in \(\hat{\C}\) and are equal to \(0\).  Thus the sequence with terms \(-u_n/u_{n-1}\) is well-defined in \(\hat{\C}\) for each \(n\in\N_0\).

A sequence \((t_n)_{n=0}^\infty\) with \(n\)th term \(t_n = -u_n/u_{n-1}\)  for some non-trivial solution \((u_n)\) is a \textit{tail sequence} of the continued fraction \(\KF(a_n/b_n)\).  
Such sequences are useful tools when discussing convergence properties of continued fractions \cite{LW1992, lorentzen2008continued}.
Suppose that \((t_n)\)  is a tail sequence such that \(t_n\neq \infty\) for each \(n\in\N_0\) then it can be shown (cf.\, \cite[Theorem 2.6]{lorentzen2008continued}) that
	\begin{equation} \label{eq: tailseqfn}
	t_0 - f_n = \frac{t_0}{\Sigma_n} \quad \text{where}\; \Sigma_n := \sum_{k=0}^n P_k \; \text{and} \; P_k := \prod_{j=1}^k \frac{b_j +t_j}{-t_j}
	\end{equation}
for each \(n\in\N_0\).
\begin{corollary}
Let \((u_n)\) be a solution to the recurrence relation \(u_n = b_n u_{n-1} + a_n u_{n-2}\) with signature \((+,-)\).  
Assume that \(u_{-1}>0\) and \((f_n)_{n=0}^\infty\) is strictly decreasing.  
Given \(N\in\N\), we have that \(t_0 < f_N\) if and only if \(u_{-1}, u_0,\ldots, u_{N}>0\).
\end{corollary}
\begin{proof}
Let us begin by assuming that for some \(N\in\N_0\), \(u_{-1}, u_0,\ldots, u_{N}>0\).
Consider \(\Sigma_N\) defined as above. 
Note that the \(j\)th factor of \(P_k\) is \((b_j + t_j)/(-t_j) > 0\) since \(u_n = b_n u_{n-1} + a_n u_{n-2} < b_n u_{n-1}\) for each \(n\in\{1,\ldots, N\}\). 
It follows from \eqref{eq: tailseqfn} that \(t_0 - f_n < 0\) for each \(n\in \{0,1,\ldots, N\}\) and so \(t_0 < f_N\).

Conversely, let us assume that \(t_0 < f_N\). 
We prove by induction that \(u_n>0\) for each \(n\in\{0,1,\ldots, N\}\).
By \eqref{eq: tailseqfn} and the fact that \((f_n)_{n=0}^\infty\) is strictly decreasing, \(0> t_0 - f_N > t_0 - f_1 = t_0/\Sigma_1 = -t_0t_1/b_1\).
We deduce that \(t_1<0\) and so \(u_1>0\).
We assume for the induction hypothesis that \(u_{-1}, u_{0},\ldots, u_{n-1}>0\).
Rearranging \eqref{eq: tailseqfn} leads us to the following
	\begin{equation*}
		t_n = -\frac{P_{n-1}(b_n+t_n)}{\frac{t_0}{t_0 -f_n} - \Sigma_{n-1}} = -P_{n-1}(b_n + t_n) \frac{(t_0-f_{n-1})(t_0 -f_{n})}{t_0(f_n-f_{n-1})}.
	\end{equation*}
	% Sign of b_n + t_n follows from a_n = t_{n-1}(b_n+t_n)
%
We deduce that \(t_n<0\) from an analysis of the signs of the terms on the right-hand side.
Thus we deduce that \(u_n>0\), as required.
\end{proof}

\begin{lemma}
If the recurrence relation \(u_n = b_n u_{n-1} + a_n u_{n-2}\) with signature \((+,-)\) admits a solution \((u_n)_{n=-1}^\infty\) with \(u_n>0\) for each \(n\in\{-1,0,1,\ldots\}\) then the associated sequence of convergents \((f_n)\) is strictly decreasing.
\end{lemma}
\begin{proof}
Recall the definition of the canonical denominators sequence \(B_n = b_n B_{n-1} + a_n B_{n-2}\) with initial conditions \(B_{-1}=0\) and \(B_0 =1\).
We claim that \(B_n >0\) for each \(n\in\N\) if and only if there is a solution \((v_n)_{n=-1}^\infty\) to the same recurrence relation such that \(v_n>0\) for each \(n\in\N_0\). 
We note that the \textit{only if} direction is trivial.

For the converse we can assume without loss of generality that \(v_{-1}>0\) and \(v_0=1\).
Since \(v_1 = b_1v_0 +a_1v_{-1} < b_1 v_0 = b_1 = B_1\), we have the inequality \(v_{1}/v_0 < B_1/B_0\).
We prove by induction that \(v_{n}/v_{n-1} < B_{n}/B_{n-1}\).
Using the induction hypothesis and the tail sequence relation we obtain the following inequality
	\begin{equation*}
		v_n/v_{n-1} = b_n + a_n v_{n-2}/v_{n-1} < b_n + a_n B_{n-2}/B_{n-1} = B_n/B_{n-1},
	\end{equation*}
which proves the claim.

From \autoref{lem: solutions} we have that \(A_n B_{n-1} - A_{n-1} B_n = -\prod_{k=1}^n (-a_k)\).
By the established claim, \(B_{n-1} B_n \neq 0\).
Thus a simple division by \(B_{n-1}B_n\) gives
	\begin{equation*}
		f_n - f_{n-1} = \frac{A_n}{B_n} - \frac{A_{n-1}}{B_{n-1}} = -\frac{\prod_{k=1}^n (-a_k)}{B_{n-1}B_{n}} < 0,
	\end{equation*}
as required.
\end{proof}
