# Supplementary material for: On Positivity and Minimality for Second-Order Holonomic Sequences
Source: arXiv:2007.12282 source file (2020-07-23)
Supplement: Supplementary file 2 [file Appendix_linear_coefficient_reductions.tex]

%\section{Interreductions of low degree holonomic sequences}\label{app:interreductions}
%In this section we consider minimality preserving reductions between holonomic sequences with
%low degree coefficients. More precisely, we consider the recurrence relation
%\eqref{eq: ogforma} with the restriction of $\deg(g_1)$, $\deg(g_2)$, $\deg(g_3)\leq 1$. As
%before, we may assume that the coefficient polynomials have constant sign. We assume that the
%considered recurrence relations admit minimal solutions.
%\todo{The purpose of this part is to reduce the number of cases we need to consider when reducing minimality to checking equality of super-generalized-periods. The main proposition says that we need only to consider the degrees triples $(1,1,1)$,  $(1,1,0)$,  $(0,1,0)$ and $(1,0,1)$. It would seem that $(1,0,1)$ is a special case of $(1,1,1)$ but I am not aware of any nice reduction for this.}

%We recall a technical property of linearly independent solutions. The proof can be assembled
%from \cite[\S IV.1.3,\S IV.1.3]{LW1992}.
%
%\begin{lemma}\label{lem:limit_of_ratios}
%For linearly independent solutions $\seq{u_n}{n}$ and $\seq{v_n}{n}$ to \eqref{eq: ogforma},
%we cannot have simultaneously $u_n = 0 = v_n$ for some $n$.
%
%If the recurrence relation \eqref{eq: ogforma} admits a minimal solution, then for any
%linearly independent pair $\seq{x_n}{n}$, $\seq{y_n}{n}$ of its solutions, the limit
%$\lim_{n\to\infty}\frac{x_n}{y_n}$ exists (in the extended complex numbers).
%\end{lemma}

%\begin{proposition}
%The problem of deciding whether a solution to \eqref{eq: ogforma} reduces as follows.
%\begin{enumerate}
%
%\item The problem of deciding whether a given solution to \eqref{eq: ogforma} with $\deg(g_3) + \deg(g_1) = 1$ is minimal reduces to the problem of deciding whether a solution to an instance of \eqref{eq: ogforma} with $\deg(g_3) = 1$ and $\deg(g_1) = 0$ is minimal.
%
%\item The problem of deciding whether a given solution to \eqref{eq: ogforma} with $\deg(g_3) + \deg(g_1) = 1$ and $\deg(g_2) = 0$ is minimal reduces to the problem of deciding whether a solution to an instance of \eqref{eq: ogforma} with $\deg(g_3) = \deg(g_2) = \deg(g_1) = 1$ is minimal.
%
%\end{enumerate}
%\end{proposition}
%
%
%\begin{proof}[Proof of \autoref{prop:linearReductions}] \hfil
%\begin{enumerate}
%\item
%This proof follows immediately from the interreduction of the recurrence relations \eqref{eq: ogforma} and \eqref{eq: sforma} described in the preliminaries.
%
%\item
%We may assume that $\deg(g_3) = 1$ and $\deg(g_1) = 0$ by the first point.
%%
%%
%Let us normalise the recurrence relation by dividing divide through by the leading coefficient of $g_3$.
%The normalised recurrence is given by
%%
%\begin{equation}\label{eq: 100}
%(n + \alpha)u_n = \beta u_{n-1} + \gamma u_{n-2}
%\end{equation}
%%
%with coefficients in \(\Q[x]\).  
%We can assume $\alpha > 1$ by taking an appropriate shift.
%%
%%
%
%Suppose that $\seq{u_n}{n}$ is a solution to \eqref{eq: 100}. 
%We observe that $\seq{u_n}{n}$ satisfies the recurrence
%%
%\begin{equation}\label{eq:modifiedRecurrence}
%(n+\alpha - 1)(n+\alpha) u_n = (2\gamma n + \beta^2 + \gamma( 2\alpha - 3))u_{n-2} - \gamma^2 u_{n-4}
%\end{equation}
%for $n\geq 3$.
%This observation follows easily from the fact  that $\beta u_{n-3} = (n+\alpha - 2) u_{n-2} - \gamma u_{n-4}$ and the following straightforward algebraic manipulations:
%%
%\begin{align*}
%(n+\alpha - 1)(n+\alpha) u_n &= (n + \alpha -1)(\beta u_{n-1} + \gamma u_{n-2})\\
%	&= \beta(n + \alpha - 1)u_{n-1} + \gamma(n + \alpha - 1) u_{n-2}  \\
%	&= (\beta^2 + \gamma(n+\alpha -1)) u_{n-2} + \beta \gamma u_{n-3}\\
%	&= (\beta^2 + \gamma(n+\alpha -1)) u_{n-2} + \gamma(n + \alpha - 2)u_{n-2} - \gamma^2 u_{n-4}\\
%	&= (2\gamma n + \beta^2 + \gamma( 2\alpha - 3))u_{n-2} - \gamma^2 u_{n-4}.
%\end{align*}
%
%Let us now define the sequence $\seq{z_n}{n}$ by $z_n = u_{2n}$ for all $n\geq 0$.
%Then
%$z_0 = u_0$ and
%\begin{equation*}
%z_1 = u_2 = \frac{1}{\alpha+2} (\beta u_1 + \gamma u_0)  = \mleft(\frac{\beta^2}{(\alpha+2)(\alpha+1)}+\gamma \mright)u_0 + \frac{\beta \gamma}{(\alpha + 2)(\alpha + 1)}u_{-1}.
%\end{equation*}
%It is clear that
%\begin{equation}\label{eq:modifiedRecurrence2}
%(2n+\alpha - 1)(2n+\alpha) z_n = (4\gamma n + \beta^2 + \gamma( 2\alpha - 3)) z_{n-1} - \gamma^2 z_{n-2}
%\end{equation}
%by \eqref{eq:modifiedRecurrence} with the mapping $n\mapsto 2n$.
%%
%This establishes a one-to-one correspondence between the solutions to
%\eqref{eq:modifiedRecurrence2} and the solutions to \eqref{eq: 100}.
%We claim that this equivalence of solutions preserves minimality.
%\todo{One computes $1+\frac{g_3(n-1)g_1(n)}{g_2(n)g_2(n-1)} = \frac{\beta^2}{2\gamma n} + \mathcal{O}(n^{-2})$, so the recurrence \eqref{eq:modifiedRecurrence2} has a minimal solution by
%\autoref{thm:contFracConvChar}, which is to be expected. The (interesting) point is that this is a repeated characteristic root case. It might be worth pointing out, perhaps not.}
%%
%%
%Observe that a solution to \eqref{eq:modifiedRecurrence2} can be transformed into a solution to the recurrence
%%
%\begin{equation*}
%(2n+\alpha - 1) v_n = (4\gamma n + \beta^2 + \gamma( 2\alpha - 3)) v_{n-1} - \gamma^2 (2n+\alpha-2)v_{n-2}
%\end{equation*}
%%
%such that this transformation preserves minimality (using the same minimality preservation reduction from \eqref{eq: ogforma} to \eqref{eq: sforma}).
%
%
%
%Let us prove the earlier claim.
%We first show that the solutions $\seq{u_n}{n}$ and $\seq{v_n}{n}$ to \eqref{eq: 100} are
%linearly independent if and only if the solutions $\seq{u_{2n}}{n}$ and $\seq{v_{2n}}{n}$ to
%\eqref{eq:modifiedRecurrence2} are linearly independent.
%If $\seq{u_n}{n}$ and $\seq{v_n}{n}$ are linearly dependent, then so are $\seq{u_{2n}}{n}$
%and $\seq{v_{2n}}{n}$. Assume thus that $\seq{u_n}{n}$ and $\seq{v_n}{n}$ are linearly independent,
%but there exists $\ell \in \R$ such that $u_{2n} = \ell v_{2n}$ for all $n\geq 0$. Hence $u_{n} - \ell v_{n} = 0$ for all even indices $n$. In particular, $\seq{u_n - \ell v_n}{n}$ is a multiple of the solution $\seq{x_n}{n}$ to \eqref{eq: 100} defined by $x_{-1} = 1$, $x_{0} = 0$. Now
%$x_{1} = \frac{\gamma}{1+\alpha}$ and
%$x_2 = \frac{\beta_1}{\alpha+2} x_1 + \frac{\gamma}{\alpha+2} x_0 = \frac{\beta \gamma}{(1+\alpha)(2+\alpha)} \neq 0 = u_2-\ell v_2$.
%This is a contradiction. We have established that $\seq{u_{2n}}{n}$ and $\seq{v_{2n}}{n}$
%are necessarily linearly independent.
%
%
%Assume now that $\seq{u_n}{n}$ is a minimal solution to \eqref{eq: 100} and let $\seq{v_n}{n}$ be a dominant solution. 
%Then % take solution $\seq{w_n}{n}$, we thus have
%\begin{equation*}
%0 = \lim_{n\to \infty}\frac{u_n}{v_n} = \lim_{n\to \infty}\frac{u_{2n}}{v_{2n}}.
%\end{equation*}
%Since $\seq{u_{2n}}{n}$ and $\seq{v_{2n}}{n}$ are linearly independent solutions to \eqref{eq:modifiedRecurrence2}, $\seq{u_{2n}}{n}$ is necessarily minimal.
%%
%%
%%
%
%Conversely, assume that the linearly independent solutions 
%$\seq{u_n}{n}$ and $\seq{v_n}{n}$ to \eqref{eq: 100} are such that $\seq{u_{2n}}{n}$ is a
%minimal solution to \eqref{eq:modifiedRecurrence2}. Then, since $\seq{v_{2n}}{n}$ is linearly
%independent to $\seq{u_{2n}}{n}$, we have $0 = \lim_{n\to\infty} \frac{u_{2n}}{v_{2n}}$. By
%\autoref{lem:limit_of_ratios} we know that the limit $\lim_{n\to\infty}\frac{u_n}{v_n}$
%exists, so $\lim_{n\to\infty}\frac{u_n}{v_n} = 0$. We have established that $\seq{u_n}{n}$ is
%a minimal solution to \eqref{eq: 100}.
%%
%
%\item 
%Let us simplify the the notation as follows. As $\alpha_1 \neq 0$, we may assume that
%$\alpha_1 = 1$ by dividing through by $\alpha_1$ if necessary. We set $\alpha:= \alpha_0$. Next, we may assume that $\beta_1 = \gamma_1$. Indeed, we consider the sequence
%$\seq{(\beta_1/\gamma_1)^n u_n}{n}$ instead, as this sequence satisfies
%the recurrence
%%
%\begin{equation*}
%(n+\alpha) v_n = \frac{\beta_1}{\gamma_1}(\beta_1 n + \beta_0)v_{n-1} + \frac{\beta_1^2}{\gamma_1^2}(\gamma_1 n + \gamma_0)v_{n-2}
%\end{equation*}
%%
%%\label{eq: lowDegreeForm}
%Clearly minimality is preserved in this translation.
%
%Finally, we may assume that $\beta_1 > 0$ by considering, if necessary, the sequence
%$\seq{(-1)^nu_n}{n}$, which satisfies the same recurrence, only $g_2$ is replaced with
%$-g_2$.
%
%\item Analogous to the above.
%
%
%\end{enumerate}
%\end{proof}
